# Supplementary material for: Spin selection rule for {\it S} level transitions in atomic rubidium under paraxial and nonparaxial two-photon excitation
Source: arXiv:2004.07685 source file (2020-04-16)
Supplement: Supplementary file 1 [file Supplemental_Material.pdf]

# Supplemental Material for

## Spin selection rule for $S$ level transitions in atomic rubidium under paraxial and nonparaxial two-photon excitation

Krishnapriya Subramonian Rajasree, Ratnesh Kumar Gupta, Vandna Gokhroo, Fam Le Kien, Thomas Nieddu,* Tridib Ray,* Síle Nic Chormaic,† and Georgiy Tkachenko

*Okinawa Institute of Science and Technology Graduate University, Onna, Okinawa 904-0495, Japan*

(Dated: April 16, 2020)

### TWO-PHOTON TRANSITION: THEORY

Consider a two-photon transition of an atom from a lower state $|g\rangle$ of energy $\hbar\omega_g$ to a higher state $|e\rangle$ of energy $\hbar\omega_e$. We assume that the transition is caused by the interaction of the atom with two light fields, labeled by the index $j = 1, 2$. We introduce the notations $\omega_j$, $\boldsymbol{\mathcal{E}}_j$, and $\mathbf{u}_j$ for the frequency, amplitude, and unit polarization vector, respectively, of the $j$th light field. The two-photon transition rate is [1]

$$P_{ge} = C\left|\frac{1}{\hbar}\sum_i\left(\frac{\langle e|\mathbf{u}_1\cdot\mathbf{d}|i\rangle\langle i|\mathbf{u}_2\cdot\mathbf{d}|g\rangle}{\omega_{ig}-\omega_2+i\Gamma_i/2} + \frac{\langle e|\mathbf{u}_2\cdot\mathbf{d}|i\rangle\langle i|\mathbf{u}_1\cdot\mathbf{d}|g\rangle}{\omega_{ig}-\omega_1+i\Gamma_i/2}\right)\right|^2, \quad (1)$$

where

$$C = \frac{1}{16\hbar^2}\frac{\Gamma}{(\omega_1+\omega_2-\omega_{eg})^2+(\Gamma/2)^2}|\boldsymbol{\mathcal{E}}_1|^2|\boldsymbol{\mathcal{E}}_2|^2. \quad (2)$$

Here, $\omega_{eg} = \omega_e - \omega_g$ is the atomic two-photon transition frequency, $\mathbf{d}$ is the atomic dipole operator, $|i\rangle$ is an intermediate state, $\omega_{ig} = \omega_i - \omega_g$ is the frequency of the atomic transition between the states $|i\rangle$ and $|g\rangle$, $\Gamma = \Gamma_e + \Gamma_g$ is the total decay rate, with $\Gamma_e$, $\Gamma_g$, and $\Gamma_i$ being the natural linewidths of the states $|e\rangle$, $|g\rangle$, and $|i\rangle$, respectively.

We find

$$P_{ge} = C|V_{eg}|^2, \quad (3)$$

where

$$V_{eg} = \sum_{K=0,1,2} V_{eg}^{(K)} \quad (4)$$

is the matrix element of the two-photon transition operator $V$ [2, 3], with the scalar ($K = 0$), vector ($K = 1$), and tensor ($K = 2$) parts given as

$$V_{eg}^{(K)} = (-1)^{K+I+J_e-M_g}\sqrt{(2F_e+1)(2F_g+1)} \times \begin{Bmatrix} F_e & K & F_g \\ J_g & I & J_e \end{Bmatrix}\alpha_J^{(K)} \times \sum_q \{\mathbf{u}_1\otimes\mathbf{u}_2\}_{Kq}\begin{pmatrix} F_e & K & F_g \\ M_e & q & -M_g \end{pmatrix}. \quad (5)$$

Here, we have introduced the notation

$$\alpha_J^{(K)} = (-1)^{K+J_e+J_g}\sqrt{2K+1}\sum_{n_iJ_i}\begin{Bmatrix} 1 & K & 1 \\ J_e & J_i & J_g \end{Bmatrix} \times \langle n_eJ_e\|\mathbf{d}\|n_iJ_i\rangle\langle n_iJ_i\|\mathbf{d}\|n_gJ_g\rangle \times\left[\frac{1}{\hbar(\omega_{n_iJ_i}-\omega_g-\omega_2+i\Gamma_i/2)} + \frac{(-1)^K}{\hbar(\omega_{n_iJ_i}-\omega_g-\omega_1+i\Gamma_i/2)}\right]. \quad (6)$$

$\alpha_J^{(K)}$ are the reduced scalar ($K = 0$), vector ($K = 1$), and tensor ($K = 2$) coefficients for the two-photon transition rate in the $J$ basis.

It is clear from Eq. (6) that, in the particular case of equal photon frequencies $\omega_1 = \omega_2$, we have $\alpha_J^{(1)} = 0$. In this case, the vector part $V^{(1)}$ of the two-photon transition operator $V$ vanishes.

The general selection rule for the electronic orbital angular momentum quantum number $L$ is that the two-photon transition can be allowed only if $|L_e - L_g| = 0, 2$. It follows from this condition that the two-photon transition can be allowed only if the initial state $|g\rangle$ and the final state $|e\rangle$ have the same parity, opposite to that of the intermediate states $|i\rangle$. This parity rule is a consequence of the odd character of the electric dipolar coupling. The parity rule for two-photon excitation is the opposite of the rule for single-photon excitation.

The general selection rule for the electronic angular momentum quantum number $J$ is that the two-photon transition can be allowed only if $|J_e - J_g| \leq 2$ [4–6]. In the case of equal photon frequencies, the transitions $J_g = 0 \to J_e = 1$ and $J_g = 1 \to J_e = 0$ are forbidden [4].

In the case where $J_e \neq J_g$, the Wigner 6-$j$ symbol in Eq. (6) for $K = 0$ is zero. This means that the coefficient $\alpha_J^{(0)}$ and the corresponding matrix element $V_{eg}^{(0)}$ of the scalar part of the two-photon transition operator $V$ vanish for $J_e \neq J_g$.

In the case where $J_e = J_g = 0$ or $1/2$, the Wigner 6-$j$ symbol in Eq. (6) for $K = 2$ is zero. This means that the coefficient $\alpha_J^{(2)}$ and the corresponding matrix element $V_{eg}^{(2)}$ of the tensor part of the two-photon transition operator $V$ vanish for $J_e = J_g = 0$ or $1/2$.

The aforementioned selection rules for the electronic angular momentum $J$ are equally true for the total an-

gular momentum $F$. However, depending on $J$, we may find additional selection rules for $F$. For instance, when $J_e = J_g = 0$ or $1/2$ and the photons have equal frequencies, we have the selection rules $F_e = F_g$ and $M_e = M_g$ [4].

The average transition rate for the transition between the hyperfine levels $F_g$ and $F_e$ is given by

$$P_{F_gF_e} = \frac{1}{2F_g+1}\sum_{M_gM_e} P_{ge}. \tag{7}$$

In the absence of a magnetic field, the level energies $\hbar\omega_g$ and $\hbar\omega_e$ do not depend on $M_g$ and $M_e$, respectively. In this case, we find

$$P_{F_gF_e} = C(2F_e+1)\sum_K \left\{ \begin{array}{ccc} F_e & K & F_g \\ J_g & I & J_e \end{array} \right\}^2 \times \frac{|\alpha_J^{(K)}|^2}{2K+1}\sum_q |\{\mathbf{u}_1\otimes\mathbf{u}_2\}_{Kq}|^2. \tag{8}$$

In the case where $J_e = J_g = 0$ or $1/2$ and $\omega_1 = \omega_2$, the two-photon operator is scalar. In this case, the transition may occur only for $F_e = F_g$ and, hence, we find

$$P_{F_gF_e} = \frac{C}{3(2J_g+1)}|\alpha_J^{(0)}|^2|(\mathbf{u}_1\cdot\mathbf{u}_2)|^2. \tag{9}$$

It is interesting to note that $P_{F_gF_e}$ does not depend on $F_g$. The line intensity $I_{F_gF_e}$ is the product of the transition rate $P_{F_gF_e}$ and the number of atoms in the initial state $|n_gJ_gF_g\rangle$. If the hyperfine sublevels of the ground state are populated according to their degeneracy, the line intensity is $I_{F_gF_e} = P_{F_gF_e}N_0(2F_g+1)/(2J_g+1)(2I+1)$, where $N_0$ is the total number of atoms in the ground state. It is clear that $I_{F_gF_e}$ is proportional to $2F_g+1$ [4].

According to Eq. (9), the dependence of the two-photon transition rate $P_{F_gF_e}$ on the polarization of the excitation light field is determined by the factor $|(\mathbf{u}_1\cdot\mathbf{u}_2)|^2$. The maximal value of this factor is 1, achieved for two fields with identical linear polarizations or opposite circular polarizations with respect to the quantization axis, $z$ (that is, opposite photon spin projections onto $z$). The minimal value of $|(\mathbf{u}_1\cdot\mathbf{u}_2)|^2$ is 0 and is achieved for two fields with orthogonal linear polarizations or identical circular polarizations with respect to $z$ (identical photon spin projections onto $z$).

## EXPERIMENTAL SITUATION WITH A NANOFIBER GUIDED FIELD

In this experiment, we study the two-photon transition $5S_{1/2}\to 6S_{1/2}$ of atomic rubidium using a single nanofiber-guided light field. The total electronic angular momentum quantum numbers of this transition are $J_e = J_g = 1/2$. The field is at exact two-photon resonance with the atom. We have $\omega_1 = \omega_2 = \omega = \omega_{eg}/2$, $\mathbf{u}_1 = \mathbf{u}_2 = \mathbf{u}$, and $\mathcal{E}_1 = \mathcal{E}_2 = \mathcal{E}/\sqrt{2}$. In this case, Eq. (9) reduces to

$$P_{F_gF_e} = \frac{1}{96\hbar^2\Gamma}|\alpha_J^{(0)}|^2|(\boldsymbol{\mathcal{E}}\cdot\boldsymbol{\mathcal{E}})|^2. \tag{10}$$

According to Eq. (10), the dependence of the two-photon transition rate $P_{F_gF_e}$ on the polarization and intensity of the field is determined by the factor

$$\xi = |(\boldsymbol{\mathcal{E}}\cdot\boldsymbol{\mathcal{E}})|^2 = |\mathcal{E}|^4|(\mathbf{u}\cdot\mathbf{u})|^2. \tag{11}$$

The field in a guided mode of a nanofiber is a structured field: it has a nonvanishing longitudinal component and an evanescent-wave nature in the fiber transverse plane [7]. Consider an elliptically polarized fundamental guided mode propagating in the $+z$ direction of the Cartesian coordinate system $(x, y, z)$. The electric part of the field in this mode is given by

$$\boldsymbol{\mathcal{E}} = (\sqrt{1+\sigma}\,\boldsymbol{\mathcal{E}}_{+1} + \sqrt{1-\sigma}\,\boldsymbol{\mathcal{E}}_{-1})/\sqrt{2}, \tag{12}$$

where $\sigma \in [-1, 1]$ is the helicity parameter [8, 9] and

$$\boldsymbol{\mathcal{E}}_p = (e_r\hat{\mathbf{r}} + pe_\varphi\hat{\boldsymbol{\varphi}} + e_z\hat{\mathbf{z}})e^{ip\varphi+i\beta z} \tag{13}$$

in cylindrical coordinates $(r, \varphi, z)$, with $p = \pm1$ being the polarization index for quasicircularly polarized fundamental guided modes [7, 10–12]. Here, $e_r$, $e_\varphi$, and $e_z$ are the reduced cylindrical components of the mode function and do not depend on $\varphi$ and $z$ [7, 10–12]. The parameter $\beta$ is the propagation constant, determined by the fiber eigenvalue equation [7]. The helicity parameter $\sigma$ is given as $\sigma = \sin 2\theta$, where $\theta$ is the angle of a quater-wave plate used in the experiment (see the main text). When we insert Eq. (13) into Eq. (12) and calculate the scalar product $(\boldsymbol{\mathcal{E}}\cdot\boldsymbol{\mathcal{E}})$, we obtain

$$(\boldsymbol{\mathcal{E}}\cdot\boldsymbol{\mathcal{E}}) = (\cos 2\varphi + i\sigma\sin 2\varphi + \sqrt{1-\sigma^2})(e_r^2+e_z^2)e^{2i\beta z} + (\cos 2\varphi + i\sigma\sin 2\varphi - \sqrt{1-\sigma^2})e_\varphi^2 e^{2i\beta z}. \tag{14}$$

The mode function components have the properties $e_r^2 = -|e_r|^2$, $e_\varphi^2 = |e_\varphi|^2$, and $e_z^2 = |e_z|^2$ [7, 10–12]. Hence, we find

$$\xi = [\sqrt{1-\sigma^2}\,(|e_z|^2 - |e_r|^2 - |e_\varphi|^2) + (|e_z|^2 - |e_r|^2 + |e_\varphi|^2)\cos 2\varphi]^2 + \sigma^2(|e_z|^2 - |e_r|^2 + |e_\varphi|^2)^2\sin^2 2\varphi. \tag{15}$$

We now consider the case of a gas of atoms around the nanofiber. We neglect the interaction and collisions between the atoms. For simplicity, we assume that the gas volume is a cylindrical shell with $z \in [0, L]$, $\varphi \in [0, 2\pi]$, and $r \in [a, r_{\max}]$. Here, $a$ is the fiber radius and $L$ and $r_{\max}$ are respectively the length and radius of the atomic cloud. The positions of the atoms in the gas are random variables. We assume that the atoms are independent from each other and have the same flat

distribution of position. We must average the factor $\xi$ over the stochastic distribution of position.

Since $\xi$ does not depend on the axial coordinate $z$, statistical averaging with respect to $z$ does not affect $\xi$. Statistical averaging with respect to the azimuthal angle $\varphi$ can be carried out by using the formulae $\langle\cos^2 2\varphi\rangle_\varphi = \langle\sin^2 2\varphi\rangle_\varphi = 1/2$ and $\langle\cos 2\varphi\rangle_\varphi = \langle\sin 2\varphi\rangle_\varphi = 0$. Here, we have introduced the notation $\langle\cdots\rangle_\varphi = (2\pi)^{-1}\int_0^{2\pi}\cdots d\varphi$ for statistical averaging with respect to $\varphi$. Hence, we find

$$\bar{\xi} = A - \sigma^2 B, \tag{16}$$

where

$$\begin{aligned} A &= \langle(|e_r|^2 + |e_\varphi|^2 - |e_z|^2)^2\rangle_r \\ &\quad + 0.5\langle(|e_r|^2 - |e_\varphi|^2 - |e_z|^2)^2\rangle_r, \\ B &= \langle(|e_r|^2 + |e_\varphi|^2 - |e_z|^2)^2\rangle_r \\ &\quad - 0.5\langle(|e_r|^2 - |e_\varphi|^2 - |e_z|^2)^2\rangle_r. \end{aligned} \tag{17}$$

Here, the notation $\bar{\xi}$ stands for the result of the statistical averaging of $\xi$ over the atomic position and the notation $\langle\cdots\rangle_r = [(r_{\max}^2 - a^2)/2]^{-1}\int_a^{r_{\max}}\cdots r dr$ is for statistical averaging with respect to the radial distance $r$.

For quasilinearly polarized fields ($\sigma = 0$), the factor $\bar{\xi}$ takes the value

$$\bar{\xi}_0 = A. \tag{18}$$

For quasicircularly polarized fields ($\sigma = \pm 1$), the factor $\bar{\xi}$ takes the value

$$\bar{\xi}_{\pm 1} = A - B. \tag{19}$$

In the case of nanofiber-mediated excitation, $\xi_{\pm 1} \neq 0$, because the field is a quasicircularly polarized guided mode and is not exactly circularly polarized.

## CALCULATION OF $\alpha_J^{(0)}$

In our experiment, the two-photon transition occurs between the ground state $|g\rangle = |5S_{1/2}\rangle$ and the excited state $|e\rangle = |6S_{1/2}\rangle$ of Rb with $\omega_1 = \omega_2 = \omega = \omega_{eg}/2$. We keep the contribution of the two most important intermediate states $|i_1\rangle = |5P_{1/2}\rangle$ and $|i_2\rangle = |5P_{3/2}\rangle$. Since the detunings are large, we neglect $\Gamma_i$. Then, Eq. (6) yields

$$\begin{aligned} \alpha_J^{(0)} = \frac{\sqrt{6}}{3\hbar}\bigg(&\frac{1}{\Delta_1}\langle e\|\mathbf{d}\|i_1\rangle\langle i_1\|\mathbf{d}\|g\rangle \\ &- \frac{1}{\Delta_2}\langle e\|\mathbf{d}\|i_2\rangle\langle i_2\|\mathbf{d}\|g\rangle\bigg), \end{aligned} \tag{20}$$

where $\Delta_1 = \omega - (\omega_{i_1} - \omega_g)$ and $\Delta_2 = \omega - (\omega_{i_2} - \omega_g)$.

With the help of the relation [2, 3]

$$\begin{aligned} \langle nLJ\|\mathbf{d}\|n'L'J'\rangle &\equiv \langle nLSJ\|\mathbf{d}\|n'L'SJ'\rangle \\ &= (-1)^{S+L+J'+1}\sqrt{(2J+1)(2J'+1)} \\ &\quad \times \begin{Bmatrix} J & 1 & J' \\ L' & S & L \end{Bmatrix}\langle nL\|\mathbf{d}\|n'L'\rangle, \end{aligned} \tag{21}$$

we find

$$\begin{aligned} \langle e\|\mathbf{d}\|i_1\rangle &= \frac{\sqrt{6}}{3}\langle 6S\|\mathbf{d}\|5P\rangle, \\ \langle e\|\mathbf{d}\|i_2\rangle &= \frac{2\sqrt{3}}{3}\langle 6S\|\mathbf{d}\|5P\rangle, \end{aligned} \tag{22}$$

and

$$\begin{aligned} \langle i_1\|\mathbf{d}\|g\rangle &= -\frac{\sqrt{6}}{3}\langle 5P\|\mathbf{d}\|5S\rangle, \\ \langle i_2\|\mathbf{d}\|g\rangle &= \frac{2\sqrt{3}}{3}\langle 5P\|\mathbf{d}\|5S\rangle. \end{aligned} \tag{23}$$

Inserting Eqs. (22) and (23) into Eq. (21) yields

$$\alpha_J^{(0)} = -\frac{2\sqrt{6}}{9\hbar}\left(\frac{1}{\Delta_1} + \frac{2}{\Delta_2}\right)\langle 6S\|\mathbf{d}\|5P\rangle\langle 5P\|\mathbf{d}\|5S\rangle. \tag{24}$$

We note that $\langle e\|\mathbf{d}\|i_1\rangle$ and $\langle e\|\mathbf{d}\|i_2\rangle$ have the same sign but $\langle i_1\|\mathbf{d}\|g\rangle$ and $\langle i_2\|\mathbf{d}\|g\rangle$ have opposite signs. Consequently, Eq. (20) yields

$$\begin{aligned} |\alpha_J^{(0)}| = \frac{\sqrt{6}}{3\hbar}\bigg|&\frac{1}{\Delta_1}|\langle e\|\mathbf{d}\|i_1\rangle\langle i_1\|\mathbf{d}\|g\rangle| \\ &+ \frac{1}{\Delta_2}|\langle e\|\mathbf{d}\|i_2\rangle\langle i_2\|\mathbf{d}\|g\rangle|\bigg|. \end{aligned} \tag{25}$$

It is known that $|\langle i_1\|\mathbf{d}\|g\rangle| = 4.253$ a.u., $|\langle i_1\|\mathbf{d}\|e\rangle| = 4.145$ a.u., $|\langle i_2\|\mathbf{d}\|g\rangle| = 6.003$ a.u., and $|\langle i_2\|\mathbf{d}\|e\rangle| = 6.047$ a.u. [13]. From these values, we find the estimates $|\langle 5P\|\mathbf{d}\|5S\rangle| = 5.202$ a.u. and $|\langle 5P\|\mathbf{d}\|6S\rangle| = 5.184$ a.u.. The lifetime of the state $6S_{1/2}$ is 45.4 ns. The lifetimes of the states $5P_{1/2}$ and $5P_{3/2}$ are 27.4 and 26 ns, respectively [13]. The energies of the states $5S_{1/2}$ and $6S_{1/2}$ are 0 and 20 132.510 cm$^{-1}$. The energies of the states $5P_{1/2}$ and $5P_{3/2}$ are 12 578.950 and 12 816.545 cm$^{-1}$ [14].

When we use the above data, we find $|\alpha_J^{(0)}| \cong 5.973 \times 10^{-38}$ kg$^{-1}$ s$^4$ A$^2$.

---

* Present address: Laboratoire Kastler Brossel, Sorbonne Université, CNRS, ENS-Université PSL, Collège de France, 4 place Jussieu, F-75005 Paris, France
† Corresponding author: sile.nicchormaic@oist.jp

[1] R. Loudon, *The Quantum Theory of Light* (Oxford: Oxford University Press, 2000).
[2] D. A. Varshalovich, A. N. Moskalev, and V. K. Khersonskii, *Quantum Theory of Angular Momentum* (Singapore: World Scientific Publishing, 2008).
[3] A. R. Edmonds, *Angular Momemtum in Quantum Mechanics* (New Jersey: Princeton University Press, 1974).
[4] G. Grynberg and B. Cagnac, Rep. Prog. Phys. **40**, 791 (1977).
[5] K. D. Bonin and T. J. McIlrath, J. Opt. Soc. Am. B **1**, 52 (1984).
[6] N. Melikechi and L. Allen, J. Opt. Soc. Am. B **3**, 41 (1986).

[7] A. W. Snyder and J. D. Love, *Optical Waveguide Theory* (New York: Chapman and Hall, 1983).

[8] K. Y. Bliokh, Y. Gorodetski, V. Kleiner, and E. Hasman, Phys. Rev. Lett. **101**, 030404 (2008).

[9] G. Tkachenko, I. Toftul, C. Esporlas, A. Maimaiti, F. Le Kien, V. G. Truong, and S. Nic Chormaic, Optica **7**, 59 (2020).

[10] F. Le Kien, J. Q. Liang, K. Hakuta, and V. I. Balykin, Opt. Commun. **242**, 445 (2004).

[11] L. Tong, J. Lou, and E. Mazur, Opt. Express **12**, 1025 (2004).

[12] F. Le Kien, T. Busch, V. G. Truong, and S. Nic Chormaic, Phys. Rev. A **96**, 023835 (2017).

[13] M. Safronova and U. Safronova, Phys. Rev. A **83**, 052508 (2011).

[14] A. Kramida, Yu. Ralchenko, J. Reader, and NIST ASD Team, NIST Atomic Spectra Database (ver. 5.7.1), [Online]. Available: `https://physics.nist.gov/asd` [2017, April 9]. National Institute of Standards and Technology, Gaithersburg, MD. (2019).
